# Supplementary material for: Anisotropic neutron spin resonance in underdoped superconducting NaFe1-xCoxAs
Source: arXiv:1409.6416 source file (2014-09-23)
Supplement: Supplementary file 1 [file supplementary_revised.pdf]

## SUPPLEMENTARY MATERIALS: ANISOTROPIC NEUTRON SPIN RESONANCE IN UNDERDOPED SUPERCONDUCTING NAFE$_{1-x}$CO$_x$AS

We used the Cryopad capability of the IN20 and IN22 spectrometers in order to ensure that the sample was in a strictly zero magnetic field environment. This avoids errors due to flux inclusion and field expulsion in the superconducting phase of the sample. Polarized neutrons were produced using a focusing Heusler monochromator and analyzed using a focusing Heusler analyzer with a fixed final wave vector at $k_f = 2.662$ Å$^{-1}$. Polarization analysis can be used to separate magnetic (e.g. spin excitations) and nuclear (e.g. phonon) scattering because the former has a tendency to flip the spin of the neutron, whereas the latter leaves the neutron spin unchanged. More specifically, the spin of the neutron is always flipped in a magnetic interaction where the neutron polarization is parallel to the wave vector transfer **Q**. We therefore describe the neutron polarization in a coordinate system where $x$ is parallel to **Q**. For convenience we then define the other orthogonal directions $y$ in the scattering plane, and $z$ out of plane [see Fig. 1(b) for a schematic of the moment directions probed]. There are then six independent configurations in which the instrument can be configured at a specific wave vector and energy point: three neutron polarization directions $x$, $y$, $z$, each which can be measured to detect neutrons that flip or do not flip their spins when scattering at the sample. The measured neutron cross-sections are labeled by the experimental configuration in which they were measured, and are written $\sigma_\alpha^{\mathrm{SF}}$, $\sigma_\alpha^{\mathrm{NSF}}$, where $\alpha$ is the neutron polarization direction ($x$, $y$ or $z$) and the superscript represents either spin-flip (SF) or non-spin flip (NSF) scattering.

Magnetic neutron scattering only probes the magnetic moment perpendicular to **Q**. The cross-sections can therefore be written in terms of $M_y$ and $M_z$ [see Fig. 1(b)], the two spatial components (perpendicular to **Q**) of the spin direction of the magnetic excitations, and in terms of the nuclear scattering strength $N$. However, a measured cross-section component on an imperfect instrument contains a leakage between SF and NSF channels due to imperfect neutron polarization. This leakage can be quantified by measuring the nuclear Bragg peak contamination into the spin flip channel, the 'instrumental flipping ratio' $R$=NSF$_\mathrm{N}$/SF$_\mathrm{N}$ (for an unpolarized instrument $R$=1, and $R \to \infty$ in the ideal case). The measured cross-section components can then be written [S1]

$$\begin{pmatrix} \sigma_x^{\mathrm{SF}} \\ \sigma_y^{\mathrm{SF}} \\ \sigma_z^{\mathrm{SF}} \\ \sigma_x^{\mathrm{NSF}} \\ \sigma_y^{\mathrm{NSF}} \\ \sigma_z^{\mathrm{NSF}} \end{pmatrix} = \frac{1}{(R+1)} \begin{pmatrix} R & R & 1 & 2R/3+1/3 & (R+1) \\ 1 & R & 1 & 2R/3+1/3 & (R+1) \\ R & 1 & 1 & 2R/3+1/3 & (R+1) \\ 1 & 1 & R & R/3+2/3 & (R+1) \\ R & 1 & R & R/3+2/3 & (R+1) \\ 1 & R & R & R/3+2/3 & (R+1) \end{pmatrix} \begin{pmatrix} M_y \\ M_z \\ N \\ \mathrm{NSI} \\ \mathrm{B} \end{pmatrix}, \tag{1}$$

where B is a background term to take account of instrumental background, which is assumed to be equal in all six cross-sections when measured at the same wave vector and energy. NSI is the nuclear spin incoherent scattering caused by moments within the nuclei of the isotopes in the sample. NSI is independent of **Q** and for the elements within this sample is negligible in magnitude compared with the nuclear incoherent cross-section $N$, and so is fixed to zero in all following calculations. Furthermore, in the case where only SF (or only NSF) cross-section components are collected, NSI would be absorbed into the B term.

By measuring $\sigma_x^{\mathrm{SF}}$, $\sigma_y^{\mathrm{SF}}$ and $\sigma_z^{\mathrm{SF}}$ at two equivalent wave vectors (i.e. $Q_2$ and $Q_4$ as described in the main text), it is possible to extract $M_a$, $M_b$, and $M_c$ via

$$\begin{cases} \sigma_x^{\mathrm{SF}}(\mathbf{Q_2}) = F^2(\mathbf{Q_2})\sin^2\theta_{\mathbf{Q_2}}\frac{R}{R+1}M_a + F^2(\mathbf{Q_2})\frac{R}{R+1}M_b + F^2(\mathbf{Q_2})\cos^2\theta_{\mathbf{Q_2}}\frac{R}{R+1}M_c + B(\mathbf{Q_2}), \\ \sigma_y^{\mathrm{SF}}(\mathbf{Q_2}) = F^2(\mathbf{Q_2})\sin^2\theta_{\mathbf{Q_2}}\frac{1}{R+1}M_a + F^2(\mathbf{Q_2})\frac{R}{R+1}M_b + F^2(\mathbf{Q_2})\cos^2\theta_{\mathbf{Q_2}}\frac{1}{R+1}M_c + B(\mathbf{Q_2}), \\ \sigma_z^{\mathrm{SF}}(\mathbf{Q_2}) = F^2(\mathbf{Q_2})\sin^2\theta_{\mathbf{Q_2}}\frac{R}{R+1}M_a + F^2(\mathbf{Q_2})\frac{1}{R+1}M_b + F^2(\mathbf{Q_2})\cos^2\theta_{\mathbf{Q_2}}\frac{R}{R+1}M_c + B(\mathbf{Q_2}), \\ \sigma_x^{\mathrm{SF}}(\mathbf{Q_4}) = rF^2(\mathbf{Q_4})\sin^2\theta_{\mathbf{Q_4}}\frac{R}{R+1}M_a + rF^2(\mathbf{Q_4})\frac{R}{R+1}M_b + rF^2(\mathbf{Q_4})\cos^2\theta_{\mathbf{Q_4}}\frac{R}{R+1}M_c + B(\mathbf{Q_4}), \\ \sigma_y^{\mathrm{SF}}(\mathbf{Q_4}) = rF^2(\mathbf{Q_4})\sin^2\theta_{\mathbf{Q_4}}\frac{1}{R+1}M_a + rF^2(\mathbf{Q_4})\frac{R}{R+1}M_b + rF^2(\mathbf{Q_4})\cos^2\theta_{\mathbf{Q_4}}\frac{1}{R+1}M_c + B(\mathbf{Q_4}), \\ \sigma_z^{\mathrm{SF}}(\mathbf{Q_4}) = rF^2(\mathbf{Q_4})\sin^2\theta_{\mathbf{Q_4}}\frac{R}{R+1}M_a + rF^2(\mathbf{Q_4})\frac{1}{R+1}M_b + rF^2(\mathbf{Q_4})\cos^2\theta_{\mathbf{Q_4}}\frac{R}{R+1}M_c + B(\mathbf{Q_4}). \end{cases} \tag{2}$$

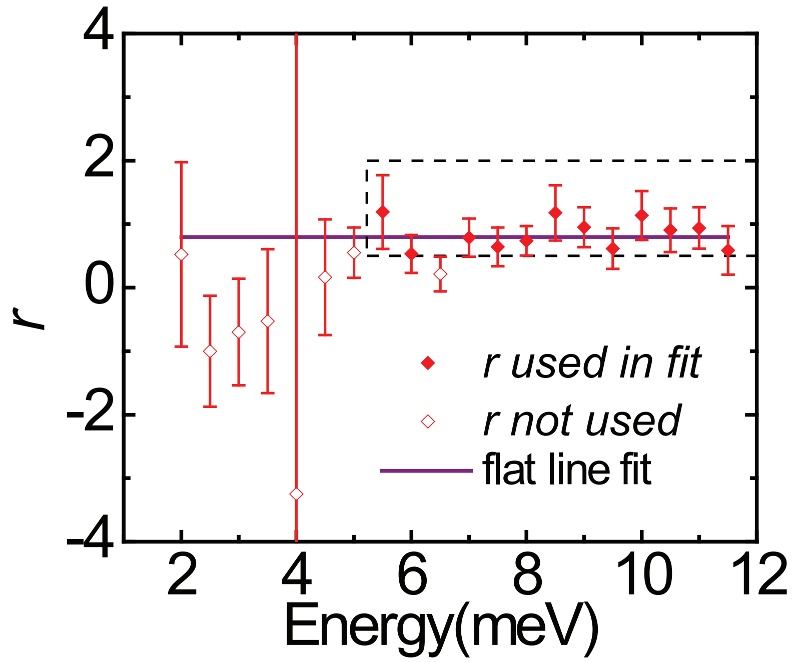


FIG. S1: $r$ obtained for the 2 K energy scans at $(1,0,0.5)$ and $(1,0,1.5)$ using Eq. (2). The flat line fit is for solid symbols satisfying $E > 5$ meV and $2 > r > 0.5$ (inside the dashed box), whereas the open symbols are not used in the fit.

where $R \approx 15$ is the spin flipping ratio determined at several nuclear Bragg peaks, $F(\mathbf{Q})$ is the magnetic form factor of $Fe^{2+}$, $B(\mathbf{Q})$ is the wave vector dependent but polarization independent background, $\theta(\mathbf{Q})$ is the angle between $\mathbf{Q}$ and [1,0,0], and $r$ is the intensity ratio factor between the two equivalent wave vectors which accounts for differences in sample illumination volume and the convolution with instrumental resolution. The six equations in Eq. (2) can be used to determine the six unknowns, $M_a$, $M_b$, $M_c$, $B(\mathbf{Q_2})$, $B(\mathbf{Q_4})$ and $r$. Solving Eq. (2) we find

$$r = \frac{F^2(\mathbf{Q_2})(\sigma_x^{\rm SF}(\mathbf{Q_4}) - \sigma_z^{\rm SF}(\mathbf{Q_4}))}{F^2(\mathbf{Q_4})(\sigma_x^{\rm SF}(\mathbf{Q_2}) - \sigma_z^{\rm SF}(\mathbf{Q_2}))} \tag{3}$$

However, when $\sigma_x^{\rm SF} \approx \sigma_z^{\rm SF}$ which corresponds to $M_b \approx 0$, $r$ can no longer be reliably determined through Eq. (3). To be able to consistently analyze all of our data to extract $M_a$, $M_b$, and $M_c$, we instead fit $r$ at points where $M_b$ is finite and extrapolate the value to points where $M_b \approx 0$. The value of $r$ is then fixed and Eq. (2) is solved as an overdetermined system of linear equations by the least squares method. Our basic assumption is that the instrumentation effect at two equivalent wave vectors should be neutron polarization and temperature independent, and change slowly with changing energy.

Using $r$ determined from Eq. (3), we find that $r$ can be well described by a constant over the energy and temperature range probed in our experiment and is therefore fit with a flat line. In Fig. S1, $r$ obtained for energy scans at 2 K for $L = 0.5, 0.15$ using Eq. (3) is fit with a flat line. Since $M_b \approx 0$ for $E \leq 5$ meV, we excluded these points in our fit. To obtain reliable results, we have further excluded points for for which $r > 2$ or $r < 0.5$. The flat line fit gives $r = 0.80 \pm 0.06$ shown as the purple line in Fig. S1. Similar procedures for the 2 K energy scans at $L = 0, 1$ gives $r = 0.80 \pm 0.08$. The 18 K energy scan for $L = 0.5, 0.15$ gives $r = 0.89 \pm 0.11$ and temperature scan at 4 meV for $L = 0.5, 0.15$ gives $r = 0.87 \pm 0.11$. We have chosen to use $r = 0.80$ to analyze all the data presented in the main text. Our results are qualitatively robust for $r$ in the range between 0.7 and 1. It should also be noted that any deviations of the magnetic form factor from that of $Fe^{2+}$ will be absorbed into the ratio factor $r$ so our analysis is independent of the values assumed for the magnetic form factor.

We have also carried out polarized INS experiments on the electron-overdoped $NaFe_{0.935}Co_{0.045}As$ ($T_c = 18$ K) [20]. Figures S2(a) and S2(b) plot the energy scans of the $\sigma_x^{\rm SF}$, $\sigma_y^{\rm SF}$, and $\sigma_z^{\rm SF}$ scattering in the superconducting ($T = 1.5$ K) and normal ($T = 25$ K) states, respectively. In unpolarized INS measurements, magnetic scattering at $T = 1.5$ K is dominated by a resonance at $E_r = 7$ meV and a spin gap below ~5 meV [20]. Below ~5 meV,

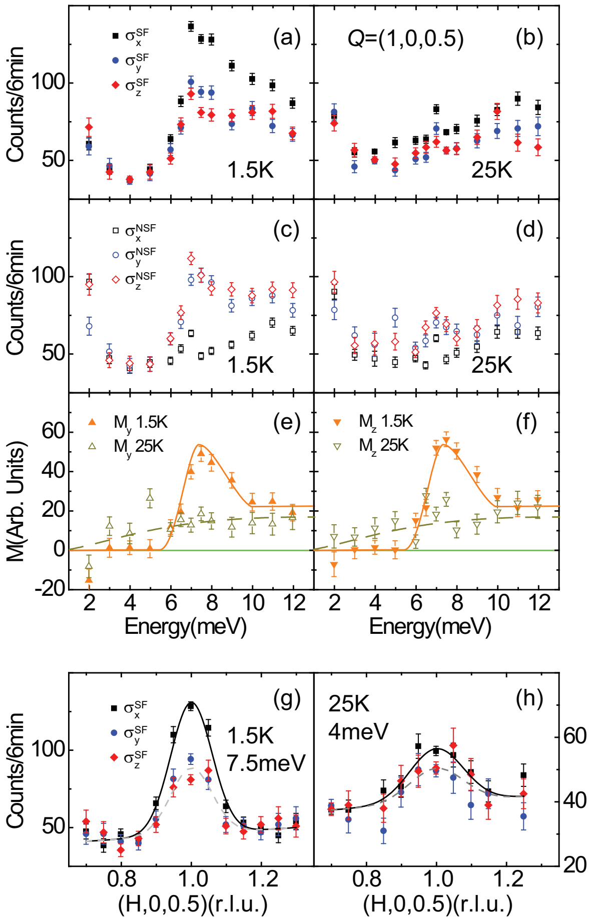


FIG. S2: (Color online) Energy dependence of the $\sigma_x^{SF}$, $\sigma_y^{SF}$, and $\sigma_z^{SF}$ at $\mathbf{Q_2} = (1, 0, 0.5)$ (a) below ($T = 1.5$ K) and (b) above ($T = 25$ K) $T_c = 18$ K for $NaFe_{0.935}Co_{0.045}As$. (c,d) Identical scans as that of (a,b) for $\sigma_x^{NSF}$, $\sigma_y^{NSF}$, and $\sigma_z^{NSF}$. Energy dependence of (e) $M_y$ and (f) $M_z$ above and below $T_c$. Constant energy scans of $\sigma_x^{SF}$, $\sigma_y^{SF}$, and $\sigma_z^{SF}$ along the $[H, 0, 0.5]$ direction at (g) $E = 7.5$ meV and 1.5 K and (h) $E = 4$ meV and 25 K. The solid lines are Gaussians fits above linear backgrounds.

we see $\sigma_x^{\rm SF} = \sigma_y^{\rm SF} = \sigma_z^{\rm SF}$ and therefore no magnetic scattering. Near $E_r = 7$ meV, we have isotropic paramagnetic scattering with $\sigma_x^{\rm SF} \approx 2\sigma_y^{\rm SF} = 2\sigma_z^{\rm SF}$ [Fig. S2(a)] [28]. Magnetic scattering in the normal state ($T = 25$ K) are gapless and have $\sigma_x^{\rm SF} > \sigma_y^{\rm SF} = \sigma_z^{\rm SF}$, again indicating isotropic paramagnetic scattering [Fig. S2(b)]. Figure S2(c) and S2(d) shows Non-Spin-Flip (NSF) scattering cross sections $\sigma_x^{\rm NSF}$, $\sigma_y^{\rm NSF}$, and $\sigma_z^{\rm NSF}$ in the superconducting and normal states, respectively. Since $\sigma_y^{\rm NSF} = \sigma_z^{\rm NSF}$ and $\sigma_x^{\rm NSF} \approx 0$, the data are consistent with isotropic paramagnetic scattering with $M_a = M_b = M_c$ [28]. Figure S2(e) and S2(f) shows energy dependence of the magnetic scattering above and below $T_c$ obtained using data in Fig. S2(a)-S2(d). We find that the normal state scattering is gapless and increases approximately linear with increasing energy. In the superconducting state, the magnetic response is composed of a spin gap and a sharp resonance at $E_r = 7$ meV. The isotropic nature of the magnetic scattering is further checked by wave vector scans along the $[H, 0, 0.5]$ direction at $E_r = 7$ meV [Fig. S2(g)] and $E = 4$ meV [Fig. S2(h)]. Since the magnetic signal above the background scattering ($b$) at both energies satisfies $\sigma_x^{\rm SF} - b \approx 2(\sigma_y^{\rm SF} - b) = 2(\sigma_z^{\rm SF} - b)$, we conclude that magnetic scattering in electron overdoped $NaFe_{0.935}Co_{0.045}As$ is isotropic at all energies and temperatures with $M_a = M_b = M_c$.

[S1] R. M. Moon, T. Riste and W. C. Koehler, Phys. Rev. 181, 920 (1969).
